# Supplementary material for: Automated Gleason Grading of Prostate Biopsies using Deep Learning
Source: arXiv:1907.07980 ancillary file (2019-07-18)
Supplement: Supplementary file 1 [file Supplementary_Information.pdf]

# Supplementary material for: Automated Gleason Grading of Prostate Biopsies using Deep Learning

**Wouter Bulten[1,*], Hans Pinckaers[1], Hester van Boven[2], Robert Vink[3], Thomas de Bel[1], Bram van Ginneken[4], Jeroen van der Laak[1], Christina Hulsbergen-van de Kaa[3], and Geert Litjens[1]**

[1]Radboud University Medical Center, Radboud Institute for Health Sciences, Department of Pathology, Nijmegen, The Netherlands
[2]The Netherlands Cancer Institute, Antoni van Leeuwenhoek Hospital (NKI-AVL), Department of Pathology, Amsterdam, The Netherlands
[3]Laboratory of Pathology East Netherlands (LabPON), Hengelo, The Netherlands
[4]Radboud University Medical Center, Radboud Institute for Health Sciences, Department of Radiology & Nuclear Medicine, Nijmegen, The Netherlands
[*]wouter.bulten@radboudumc.nl

## Contents

**1 Supplementary figures** **2**
1.1 Study flow chart . . . 2
1.2 Case distribution test set . . . 3
1.3 Confusion matrices experts with consensus on test set . . . 4
1.4 Confusion matrices experts with consensus on observer set . . . 4
1.5 Gleason score agreement of deep learning system versus panel . . . 5
1.6 Accuracy deep learning system accuracy versus panel . . . 5
1.7 Grade group agreement between pathologists . . . 6
1.8 Test set cases with Gleason overlays . . . 7
1.9 Grade group agreement of deep learning system versus panel . . . 8
1.10 Confusion matrix TMA set . . . 9

**2 Supplementary tables** **10**
2.1 Excluded cases from test set . . . 10
2.2 Consensus meeting cases and final consensus score . . . 11

**3 Supplementary methods** **12**
3.1 Tumor detection system . . . 12
3.2 Epithelium segmentation system . . . 12
3.3 Determining the Gleason grade group for a new specimen . . . 12
3.4 CycleGAN for style transformation and application to external data . . . 12

**Supplementary references** **13**

# 1 Supplementary figures

## 1.1 Study flow chart

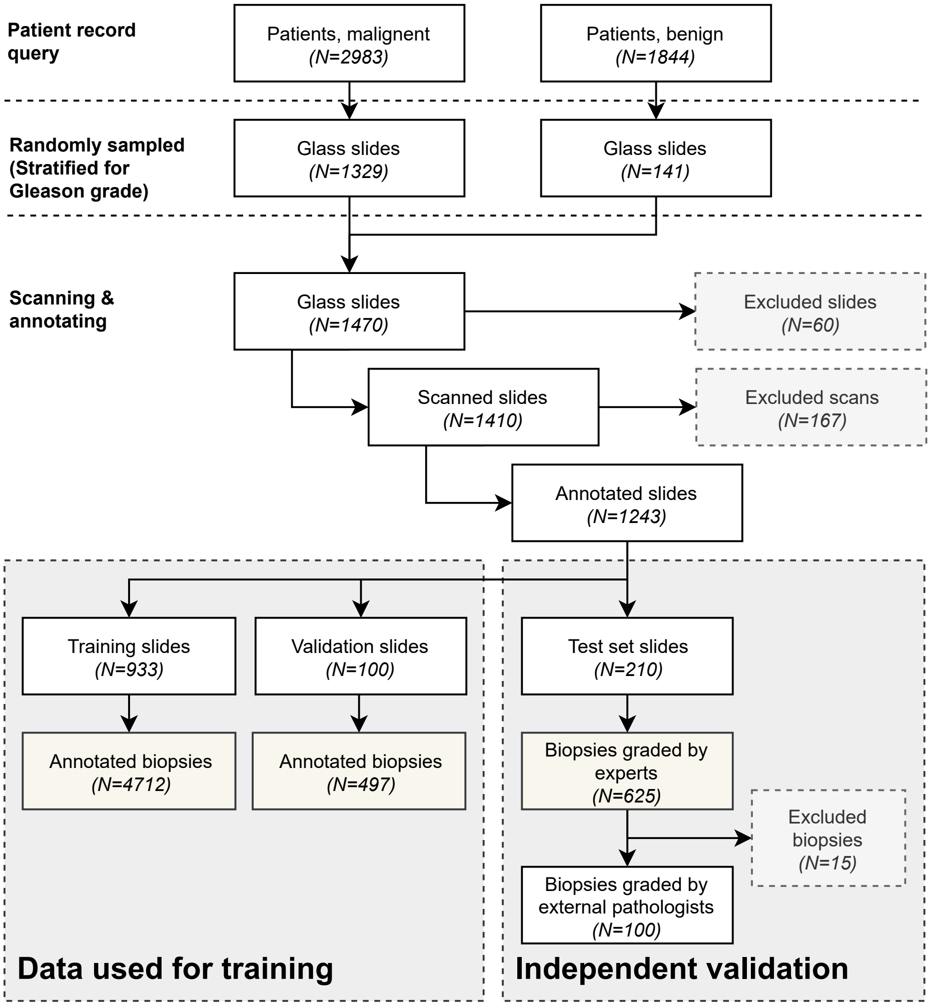


**Supplementary Figure 1.** Overview of the data that was included in the study for both training and validation of the deep learning system.

## 1.2 Case distribution test set

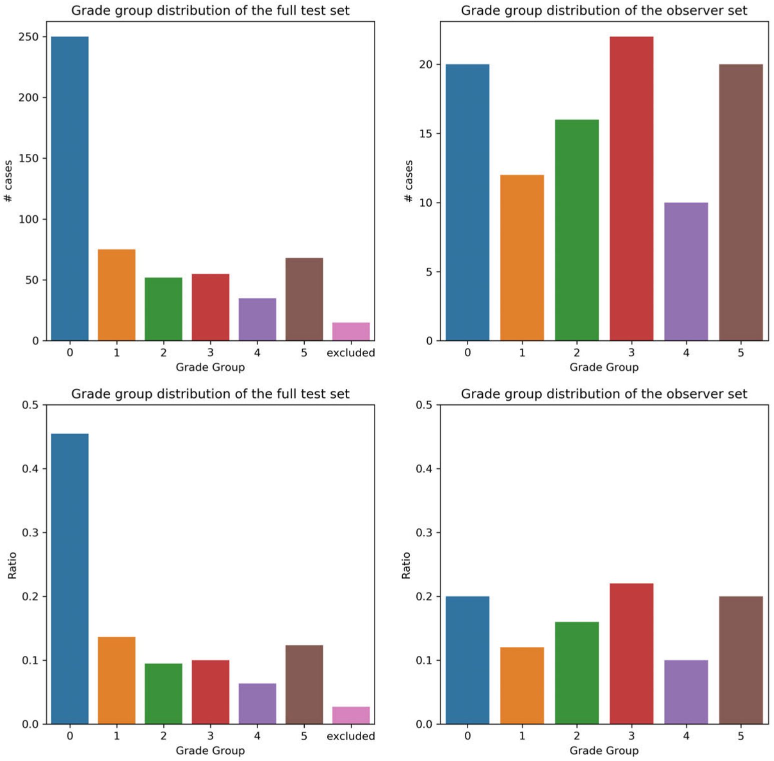


**Supplementary Figure 2.** Grade group distribution of the cases of the full test set (left) and the observer set that was presented to the external panel (right). Cases for the observer set were sampled from the test set. Top row shows the number of cases in each set, the bottom row the ratio. Both sets differ in distribution: for the full test we opted for a distribution that is close to clinical practice by including a large set of negative cases. For the observer set we included a comparable number of cases from all grade groups.

## 1.3 Confusion matrices experts with consensus on test set

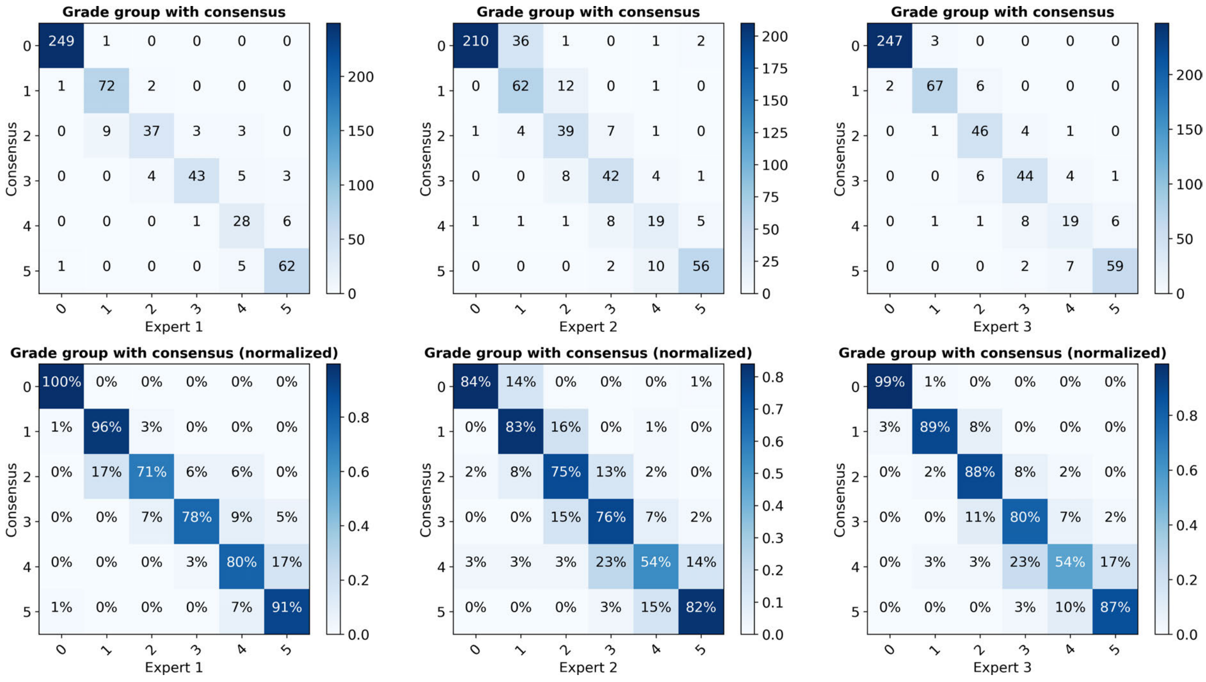


**Supplementary Figure 3.** Confusion matrices for the three expert pathologists on the test set. The original scores of the pathologists (from round 1) are compared with the final consensus scores.

## 1.4 Confusion matrices experts with consensus on observer set

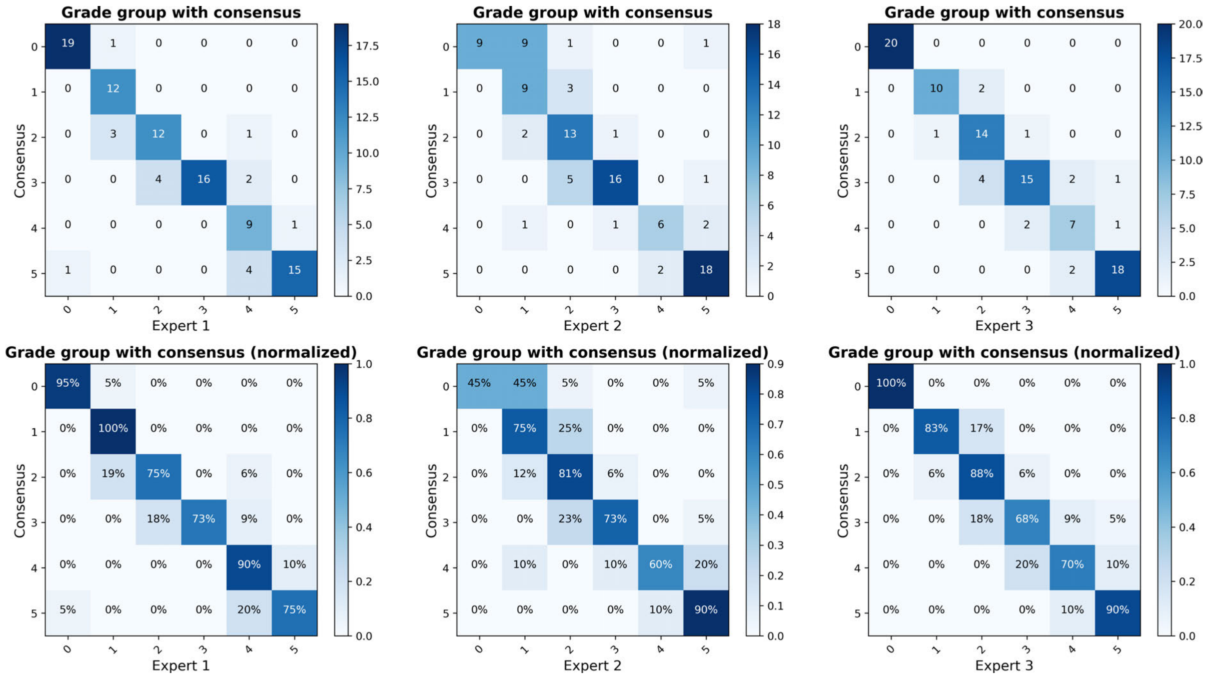


**Supplementary Figure 4.** Confusion matrices for the three expert pathologists on the observer set. The original scores of the pathologists (from round 1) are compared with the final consensus scores.

## 1.5 Gleason score agreement of deep learning system versus panel

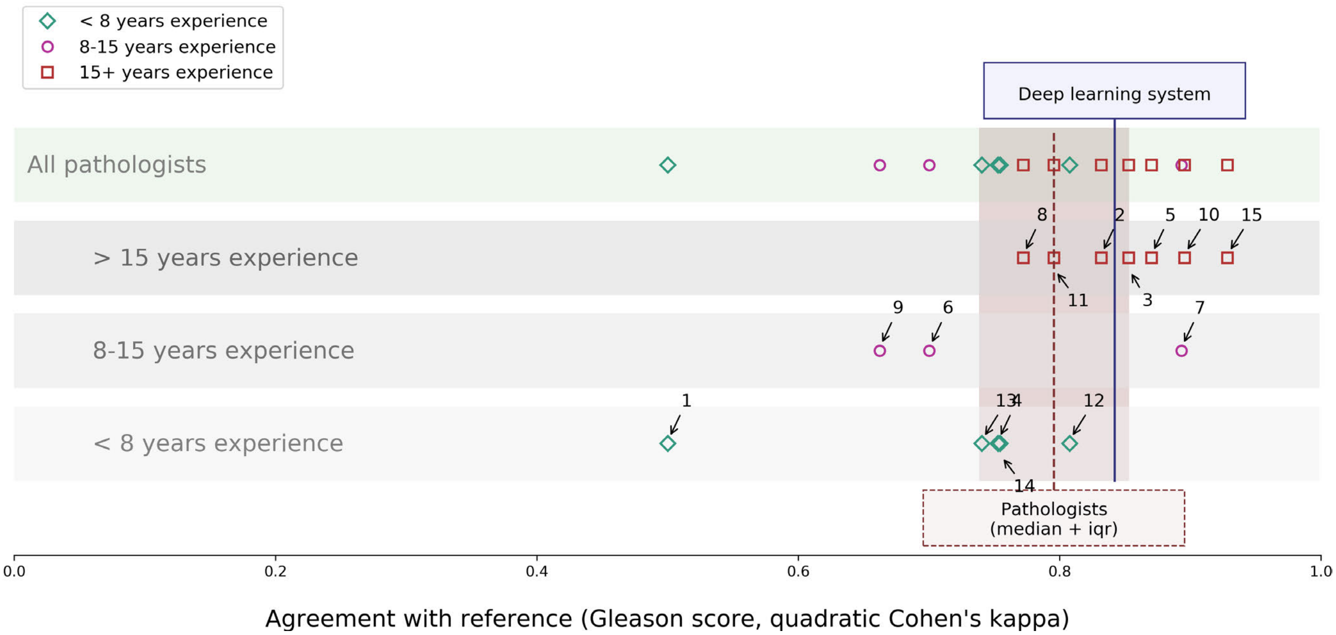


**Supplementary Figure 5.** Agreement with the reference standard on Gleason score (sum of both primary and secondary pattern) of both the panel members and the deep learning system.

## 1.6 Accuracy deep learning system accuracy versus panel

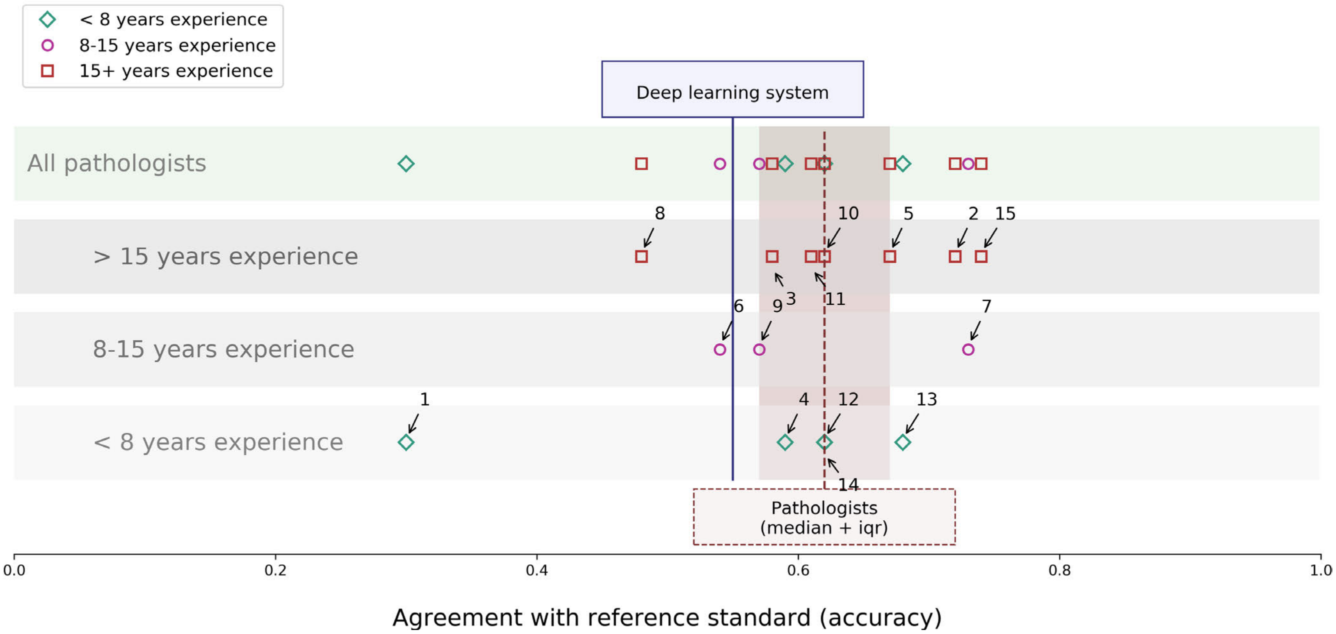


**Supplementary Figure 6.** Grade group accuracy compared to the reference standard of both the panel members and the deep learning system.

## 1.7 Grade group agreement between pathologists

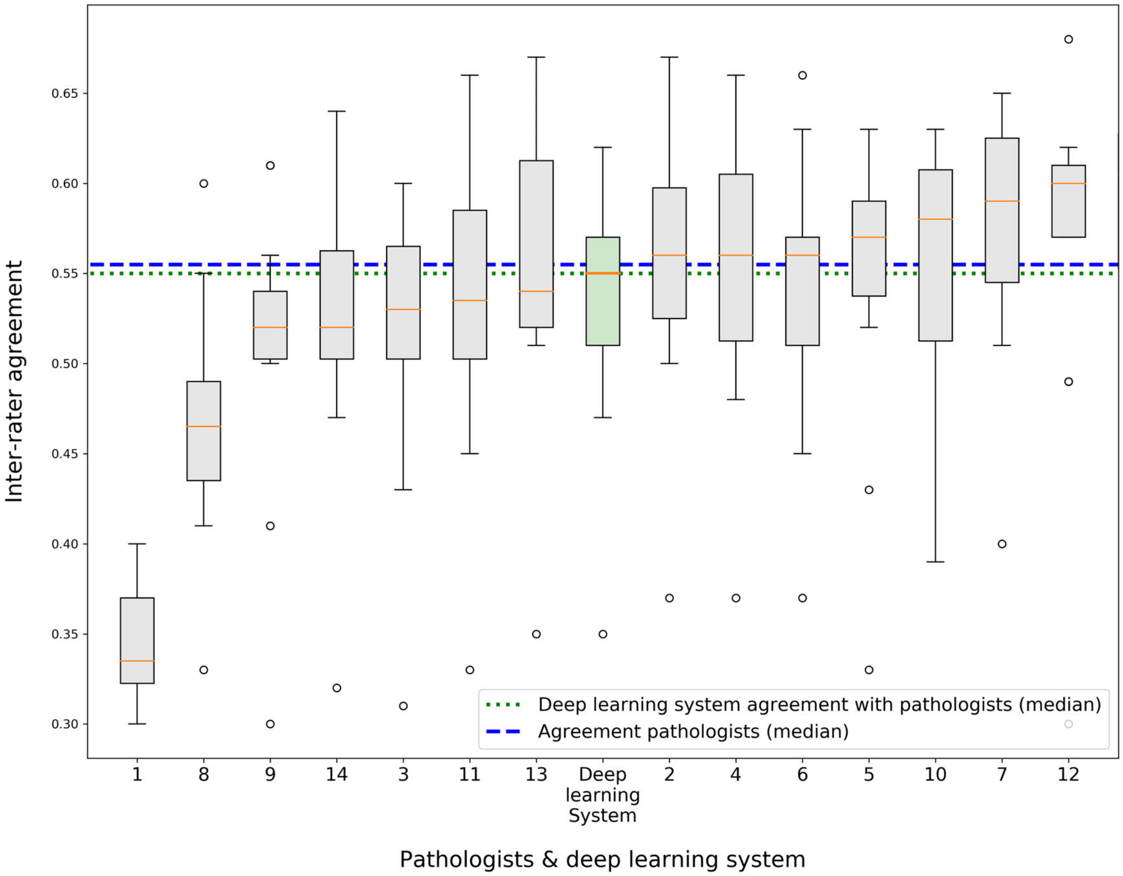


**Supplementary Figure 7.** Inter-rater agreement (non-weighted accuracy measure) between external pathologists. For each pathologist the agreement with each other pathologist was calculated. Additionally displayed is the agreement of the deep learning system with all pathologists.

## 1.8 Test set cases with Gleason overlays

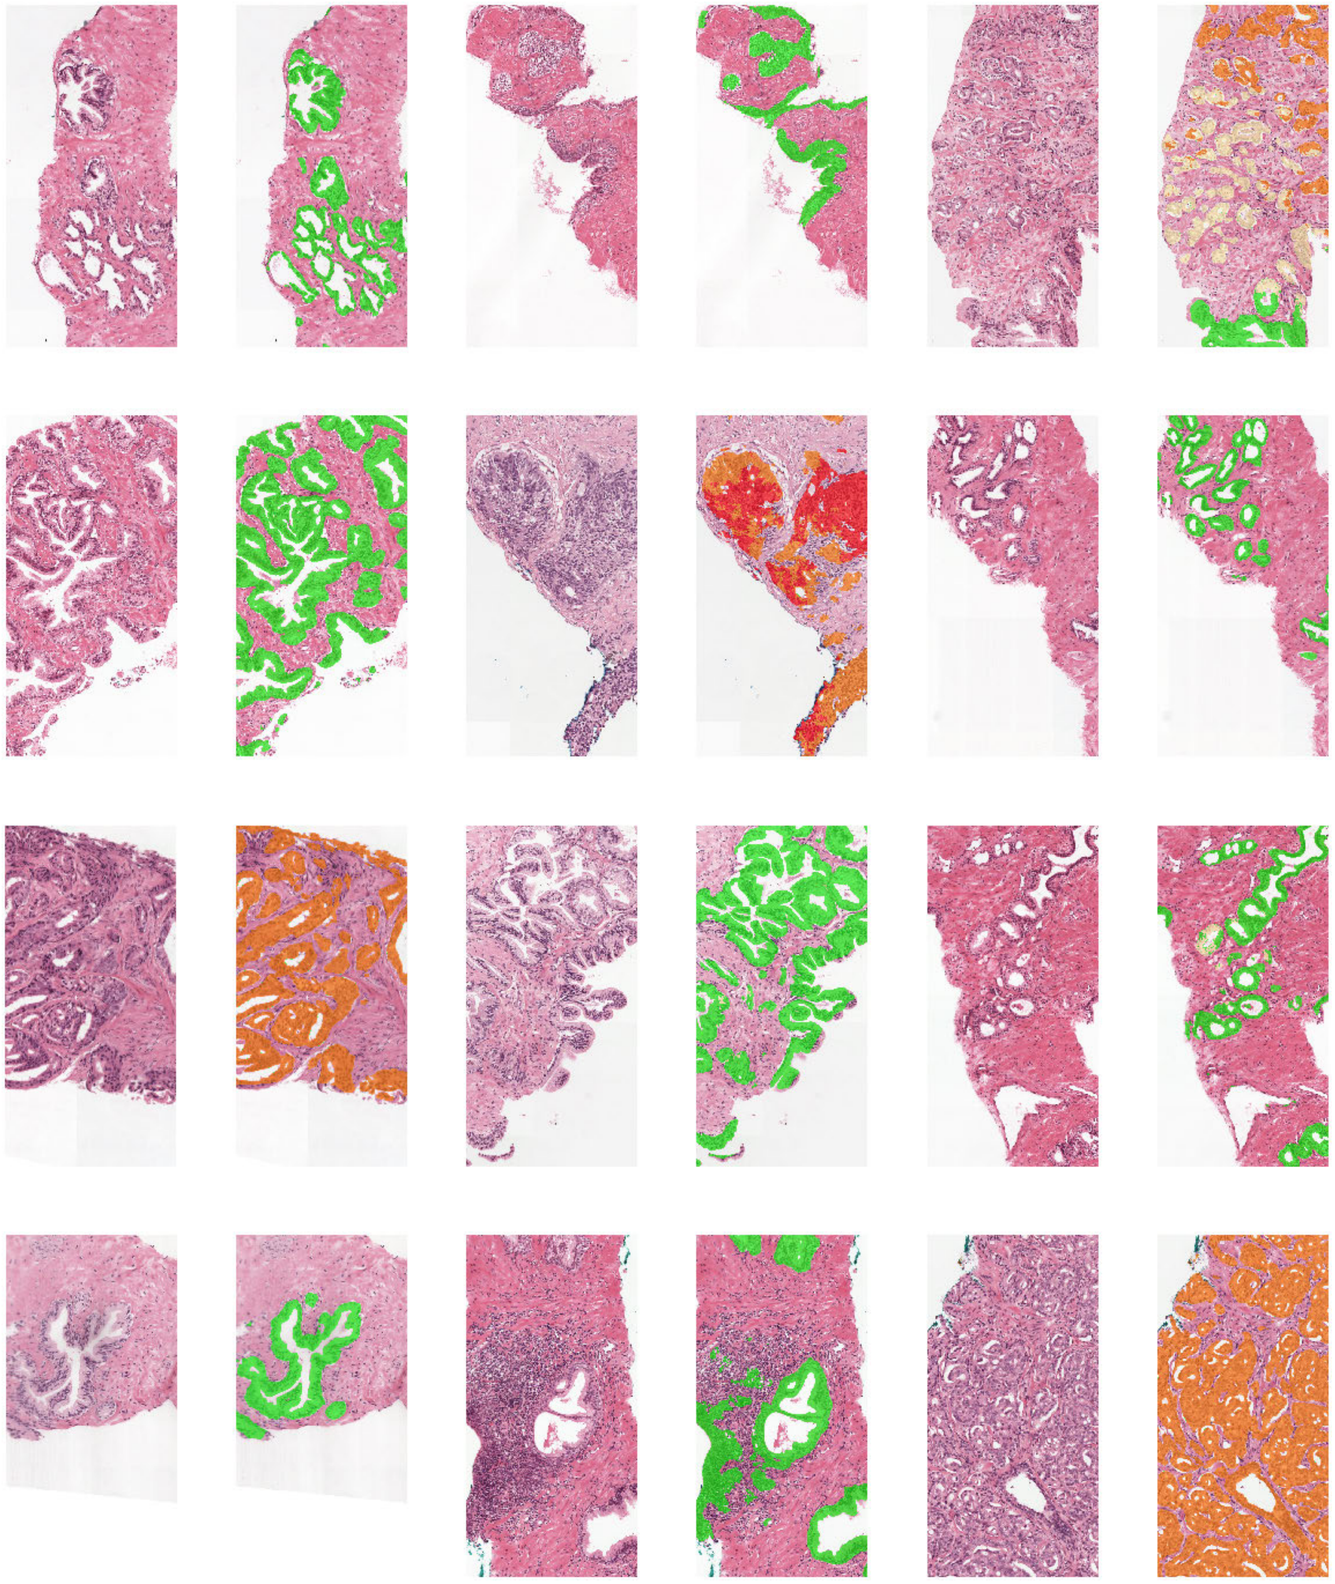

**Supplementary Figure 8.** Random cases selected from the test set. The overlay shows the predictions of the deep learning system: benign tissue (green), Gleason 3 (yellow), Gleason 4 (Orange) and Gleason 5 (red).

### 1.9 Grade group agreement of deep learning system versus panel

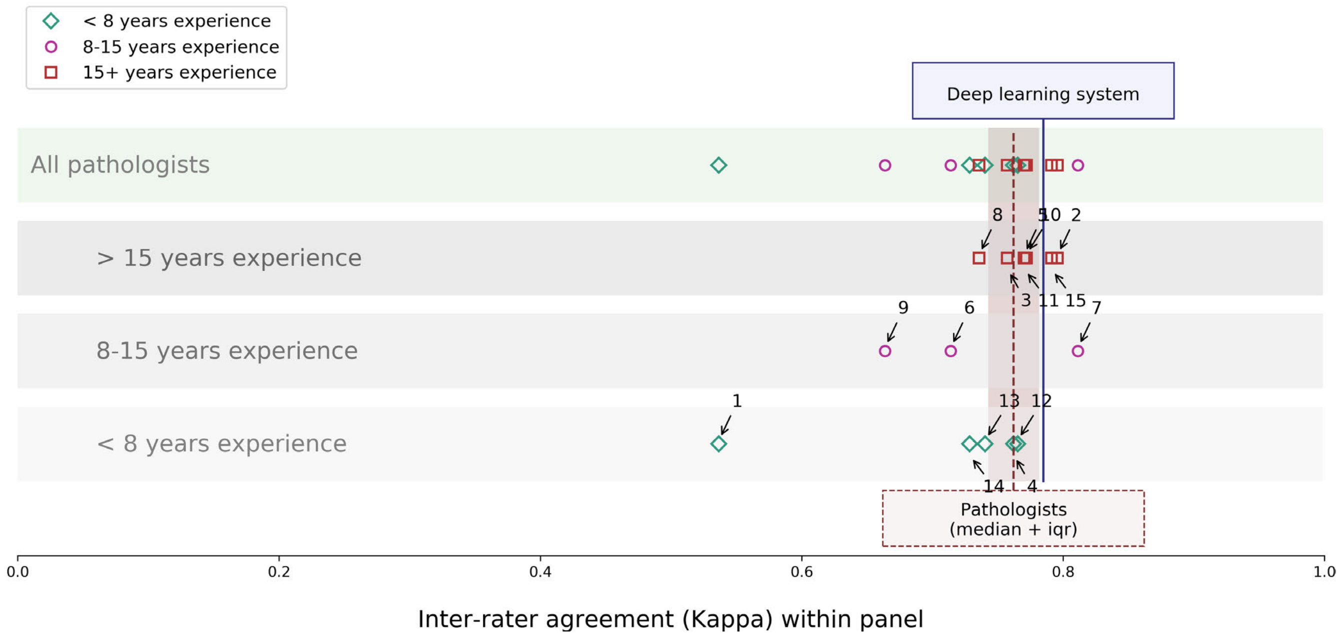


**Supplementary Figure 9.** Median inter-rater agreement of panel members with each other, compared to the median agreement of the network with the panel. The reference standard, set by the three experts, was not used in this analysis.

### 1.10 Confusion matrix TMA set

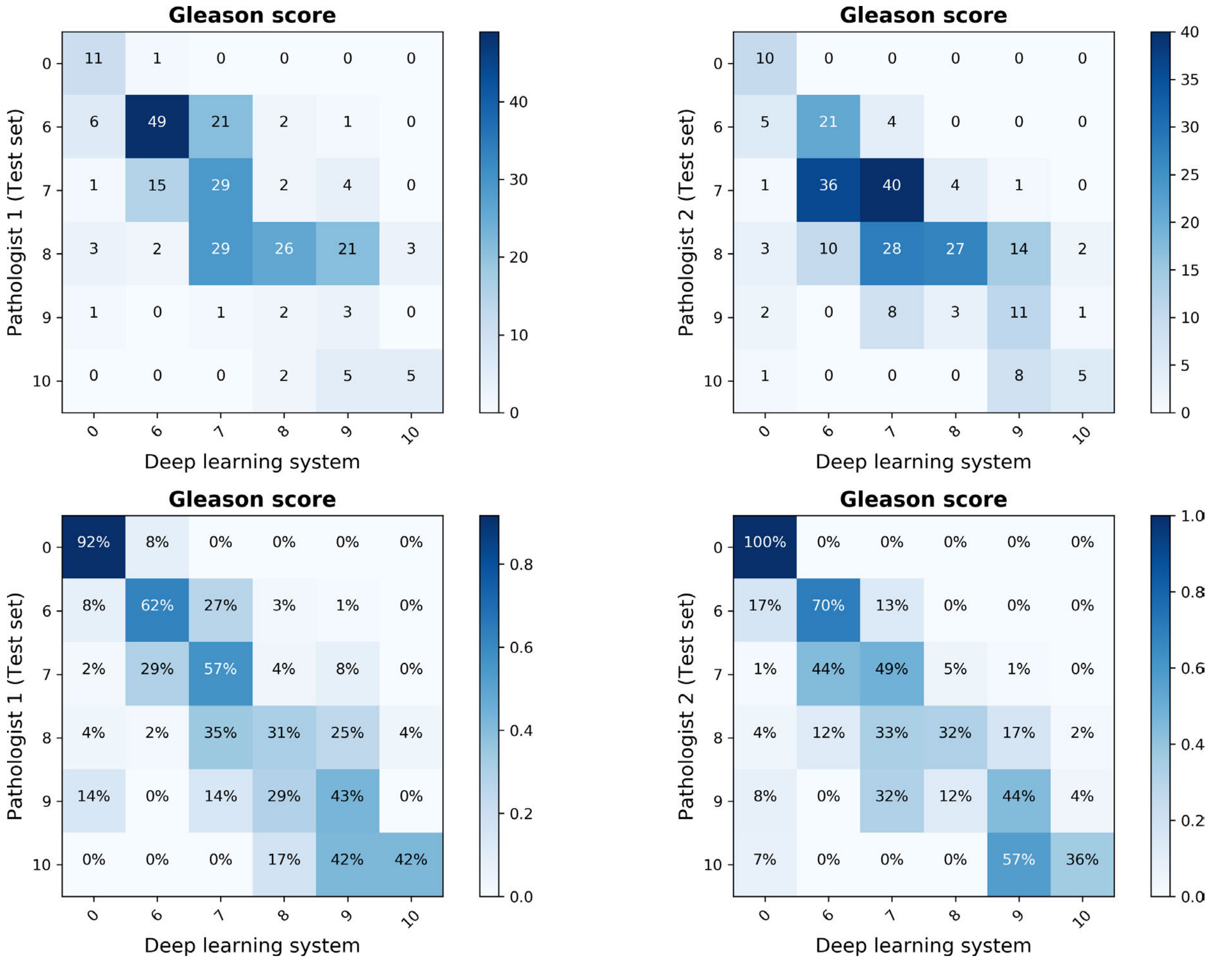


**Supplementary Figure 10.** Confusion matrices for the external test set of tissue micro arrays. The first column shows the predictions of the deep learning system compared to the first pathologists. The second column shows the results with respect to the second pathologist.

## 2 Supplementary tables

### 2.1 Excluded cases from test set

**Supplementary Table 1.** Excluded cases from the test set. 15 cases were excluded from the test set by at least one of the expert pathologists.

| Case ID | Reason for exclusion |
|---|---|
| 44 | Tumour area to small to grade. |
| 55 | Unsharp. |
| 129 | Error in loading file. |
| 161 | Possibly pretreated, IHC needed. |
| 184 | IHC needed. |
| 185 | Mechanically damaged. |
| 248 | Too small to grade. |
| 247 | IHC needed. |
| 250 | Need serial sectioning. |
| 281 | Image quality too low for grading. |
| 315 | Out of focus. |
| 380 | Unsharp. |
| 406 | Unsharp. |
| 473 | Unsharp. |
| 497 | Difficult to grade because of small amount of tumor. |

### 2.2 Consensus meeting cases and final consensus score

**Supplementary Table 2.** Cases from the test set of which there was no consensus after the second round. These cases were discussed in a consensus meeting with the three experts. For some of the cases the experts indicated that IHC would have been ordered in clinical practice.

| Case ID | Expert 1 | Expert 2 | Expert 3 | Final consensus label | Comments |
|---|---|---|---|---|---|
| 14 | negative | 5+4 | 5+4 | 5+4 | IHC required to confirm. |
| 21 | negative | 3+3 | negative | negative | |
| 249 | negative | 5+5 | negative | negative | IHC required to confirm. |
| 257 | 3+5 | 3+4 | 3+4 | 4+3 | |
| 333 | negative | 3+3 | negative | negative | |
| 388 | 3+5 | 3+4 | 3+4 | 3+4 | Possible 3+5. |
| 482 | 3+3 | 3+3 | negative | negative | IHC required to confirm. |
| 2 | 4+5 | 4+3 | 4+4 | 4+4 | |
| 15 | 4+5 | 4+5 | 4+3 | 4+5 | |
| 106 | 4+5 | 4+3 | 4+3 | 4+3 | |
| 138 | 4+5 | 4+3 | 4+3 | 4+3 | |
| 170 | negative | 5+5 | negative | negative | |
| 211 | 4+5 | 4+3 | 4+3 | 4+3 | |
| 227 | negative | 3+3 | negative | negative | |
| 272 | negative | 3+3 | 3+3 | negative | IHC required to confirm. |
| 284 | negative | 3+3 | negative | negative | |
| 290 | 3+5 | 3+3 | 4+3 | 3+4 | Volume percentage too low to be certain. |
| 306 | negative | 3+3 | 3+3 | negative | IHC required to confirm. |
| 317 | 4+5 | 4+3 | 4+3 | 4+3 | IHC required to rule out mechanical damage. |
| 356 | 3+3 | 3+4 | 4+3 | 3+3 | Volume percentage too low to be certain. |
| 369 | 3+5 | 3+4 | 3+5 | 3+4 | Possible 3+5. |
| 372 | negative | 3+3 | negative | negative | IHC required to confirm. |
| 386 | negative | 3+3 | 3+3 | negative | IHC required to confirm. |
| 390 | negative | 3+3 | negative | negative | IHC required to confirm. |
| 414 | 5+4 | 4+3 | 4+3 | 4+3 | |
| 544 | 4+5 | 4+3 | 4+3 | 4+4 | |
| 545 | 5+4 | 4+3 | 4+3 | 4+5 | |

# 3 Supplementary methods

## 3.1 Tumor detection system

A previously developed tumor detection system was applied[1] to outline tumor areas in our training set. To train this tumor detection system, a pathologist in training, supervised by an experienced uropathologist, outlined tumor regions in 100 prostate biopsies. Most of these biopsies were low grade: 52 benign, 11 grade group 1, 23 grade group 2, seven grade group 3, five grade group 4, and two biopsies grade group 5. The biopsies used for the development of the tumor detection system were independent of the biopsies used in the current study.

Patches were extracted from the 100 biopsies and used to train the system (pixel resolution of $1.92\mu m$). The tumor detection system achieved an AUC of 0.99 in discriminating benign from malignant biopsies on a separate test set of 75 biopsies.

After training the system was applied as a fully convolutional network to all biopsies of the current study. This procedure resulted in a rough outline of tumor regions.

## 3.2 Epithelium segmentation system

A previously developed epithelium segmentation system[2] was used to refine the tumor outlines generated by the tumor detection system. The epithelium segmentation system was developed using 102 prostatectomy tissue sections. The tissue sections were stained with H&E and subsequently restained with P63 and CK8/18 immunohistochemistry (IHC) markers to highlight epithelial structures. Each H&E and IHC pair were subsequently co-registered.

An initial deep learning system was trained on a subset of the IHC slides that were preprocessed with color deconvolution. This trained system was then applied to all IHC slides in the training set, forming a reference standard for the final system. This automated labeling method made sure that even poorly differentiated Gleason 5 areas were precisely annotated.

The final epithelium segmentation system was trained on the H&E slides using the automatically generated reference standard. A five-level-deep U-Net[3] was used as the network architecture with patches extracted at a pixel resolution of $0.98\mu m$. The system achieved a high segmentation performance (F1 score of 0.893) and was able to segment both intact glands and individual malignant epithelial cells.

## 3.3 Determining the Gleason grade group for a new specimen

Our deep learning system determines the Gleason grade group for a biopsy in two steps. First, our trained U-Net is applied to the scanned tissue of the biopsy. This procedure results in a label for each pixel of the image: background, stroma, benign epithelium, Gleason 3, Gleason 4, or Gleason 5. The frequency of each label can then be counted. Biopsies can differ vastly in size and in the amount of epithelial tissue that is present. To account for this difference, the values for the three Gleason growth patterns are normalized based on the sum of benign and malignant epithelial tissue. By normalizing we obtain a volume estimate of the tumor that is independent of the size of the biopsy.

The volume percentages are used to determine the grade group of the biopsy. First, we determine whether a biopsy is malignant or benign. Based on the tuning set we classify a biopsy as malignant if at least 10% of the epithelial tissue is predicted as cancer by the system. For malignant biopsies, we then determine the Gleason score. The growth pattern that has the largest volume is taken as the primary component. If there are other growth patterns present, with a volume of at least 7%, the most aggressive component is used as the secondary pattern. The 7% cut-off was determined automatically based on the tuning set. Note that this procedure differs between prostatectomies and biopsies. For prostatectomies, the secondary pattern is always the second-largest growth pattern, regardless of aggressiveness.

The predicted Gleason score is used to determine the grade group. A Gleason score 3+3 is mapped to group 1; Gleason score 3+4 is mapped to group 2; Gleason score 4+3 is mapped to group 3; Gleason scores 3+5, 4+4 and 5+3 are mapped to group 4; and higher scores are mapped to Gleason 5.

## 3.4 CycleGAN for style transformation and application to external data

We used a cycle-consistent generative adversarial network (CycleGAN)[4] system to facilitate stain transformation on the external dataset of tissue microarrays. In a CycleGAN setup, two separate networks are trained to perform a transformation from one stain to the other, while retaining the structural information of the tissue. We used a previously developed CycleGAN setup that was developed for transformation of histopathological tissue[5].

To train the CycleGAN system, we sampled patches from the training set of the Radboud data and used the full external dataset. Before inference with the Gleason deep learning system, we applied the CycleGAN network and Gaussian blurring on the whole external dataset. The CycleGAN network was implemented in TensorFlow[6].

## Supplementary references


1. Litjens, G. *et al.* Deep learning as a tool for increased accuracy and efficiency of histopathological diagnosis. *Nat. Sci. Reports* **6**, 26286, DOI: 10.1038/srep26286 (2016).
2. Bulten, W. *et al.* Epithelium segmentation using deep learning in H&E-stained prostate specimens with immunohistochemistry as reference standard. *Sci. Reports* **9**, 1–7, DOI: 10.1038/s41598-018-37257-4 (2019).
3. Ronneberger, O., Fischer, P. & Brox, T. U-net: Convolutional networks for biomedical image segmentation. In *Medical Image Computing and Computer-Assisted Intervention*, vol. 9351 of *Lecture Notes in Computer Science*, 234–241 (2015).
4. Zhu, J.-Y., Park, T., Isola, P. & Efros, A. A. Unpaired image-to-image translation using cycle-consistent adversarial networks. In *Proceedings of the IEEE international conference on computer vision*, 2223–2232 (2017).
5. de Bel, T., Hermsen, M., Kers, J., van der Laak, J. & Litjens, G. Stain-transforming cycle-consistent generative adversarial networks for improved segmentation of renal histopathology. In Cardoso, M. J. *et al.* (eds.) *Proceedings of The 2nd International Conference on Medical Imaging with Deep Learning*, vol. 102 of *Proceedings of Machine Learning Research*, 151–163 (PMLR, London, United Kingdom, 2019).
6. Abadi, M. *et al.* TensorFlow: Large-scale machine learning on heterogeneous systems (2015). Software available from tensorflow.org.
